# Supplementary material for: Industry Influence in High-Profile Social Media Research
Source: arXiv:2601.11507 ancillary file (2026-01-16)
Supplement: Supplementary file 1 [file SI.pdf]

Supplementary Materials for:
# *Industry Influence in High-Profile Social Media Research*

Joseph Bak-Coleman[1,2,3,4,5*], Jevin West[6,7], Cailin O'Connor[8,9], and Carl T. Bergstrom[1,2,7]

[1]Department of Biology, University of Washington, Seattle, WA, USA
[2]Santa Fe Institute, Santa Fe, NM, USA
[3]Centre for the Advanced Study of Collective Behavior, University of Konstanz, Germany
[4]Department of Collective Behavior, Max Planck Institute of Animal Behavior, Germany
[5]Berkman Klein Center, Harvard University, Cambridge, MA, USA
[6]Information School, University of Washington, Seattle, WA, USA
[7]Center for an Informed Public, University of Washington, Seattle, WA, USA
[8]Department of Logic and Philosophy of Science, UC Irvine, Irvine, CA, USA
[9]Center for Socially Engaged Philosophy, UC Irvine, Irvine, CA, USA

*To whom correspondence should be addressed; E-mail: jbakcoleman@gmail.com

## S1 Data Collection

We define high-profile journals as *Nature*, *PNAS*, and *Science*, alongside their typical transfer journals of *PNAS Nexus*, *Science Advances*, *Nature Communications*, and *Nature Human Behavior*. We focus on these journals as they are interdisciplinary and high profile, such that they would be read more broadly than high-profile journals within a given discipline.

We queried OpenAlex on November 6th, 2025 using for all papers published after 2010 containing *"social media OR WhatsApp OR Instagram OR Facebook OR Youtube OR Linkedin OR Twitter"* [1]. We also limited our search to records labeled by OpenAlex as "articles". This limits our corpus to papers either about one of the four firms' products or about the domain in which these products compete (i.e., social media). In total this identified

728 candidate papers. We then removed incomplete records that lacked authors, affiliations, or referenced works. This filtering was necessary as each of the observables were required for our analysis and it filtered some news, comments and other informal records. This left 353 candidate records.

However, this remaining corpus contained a mixture of research that was about social media as well as work that merely mentioned it in passing or leveraged it to address other questions. To eliminate off-topic research, we constructed a bibliographic coupling network. From this, we we extracted the $K$-Truss, which is a relaxation of $K$-cliques that identifies the maximal subgraph such that all remaining nodes are a part of $K-2$ closed triangles (here, $K=4$). For each of these remaining records, we manually examined the PDF versions of the manuscripts to check competing interests statements, funding statements and acknowledgments for indications of disclosable interests to Meta, Google, Twitter, Microsoft or related entities (e.g. DeepMind, Jigsaw).

## S2 Disclosable Interest Identification

From our corpus, we extracted all of the unique authors to form our dataset of 1210 authors. For each author, we began by checking for prior employment. To do so, we examined OpenAlex records for years in which they published with an affiliation to one of our four firms. As OpenAlex occasionally produces affiliation false-positives, we eliminated any authors for which an affiliation was identified in only a single year. This is a conservative choice intended to reduce false positives, potentially at the cost of false negatives. Finally, we manually examined remaining authors to ensure they were indeed formally affiliated with the firm at some point in time. We note that our employment method many miss some authors who were employed but did not publish, or only published within a single year.

Next we extended our employment disclosable interests for Meta specifically, as they offer a fellowship which generally includes two-year stipend received by individuals rather than as research funding. To do so, we extracted all of the names from past fellows on Meta's research blog [1]. We matched the listed names to records for OpenAlex, and included the two years after the announcement year given the typical duration of the fellowship.

To identify prior collaboration, we queried OpenAlex for all publications with an institution affiliated with our firms. For Google, this included

[1] `https://research.facebook.com/fellows/`

Google, Deepmind, and Alphabet. For Meta, this included Facebook as well as “Menlo School” which is a a private high school we identified as the frequently recorded affiliation for Meta employees. The actual Menlo School, is a high school and has produced very few research publications. For Microsoft we included Microsoft, Microsoft Research and OpenAI with whom they have a significant financial association. Twitter was only listed in OpenAlex as Twitter.

To ensure collaborations were relevant to social media and reduce false positives, we limited this search to industry co-authored papers matching our corpus search string above. A collaboration disclosable interest was defined as being a co-author on any of these industry co-authored papers. Our definition here is conservative as well, excluding informal collaboration, advisory roles, or any other form of collaboration that did not produce academic research.

We identified funding in two distinct ways. First, we queried OpenAlex for all research identifying one of our four firms as a funder. We excluded any paper with more than 10 authors, to avoid megastudies leading to many assignments of disclosable interests. However, funding links on OpenAlex are per-paper, not per-author. As such, we manually reviewed all funding ties to ensure authors identified in our dataset were not tied to their co-authors sources of funding. To do so, we first checked the funding statements to see if the author was explicitly (e.g. “[Author] is grateful for funding from [company]”) or implicitly (e.g. “We are grateful for funding from [company]”). When there was uncertainty, we examined third sources (C.V.’s, author websites) to ascertain if they received funding from that company, in that time-frame. We excluded any cases which we could not verify, or for which the funding was clearly received by a co-author. For each funding disclosable interest identified in this manner, we counted the year before publication and the year of publication to account for the time in which the research was being conducted.

We extended these funding disclosable interests by matching authors in our database to publicly available funding awards from Google[2] and Meta’s RFPs [3]. Here, we included the year awarded and the subsequent year to allow for project duration. Although projects may last longer than a year, we chose this as a conservative estimate of project duration. We note that X and Microsoft do not have available information on similar RFPs, such that

[2] `https://research.google/programs-and-events/google-academic-research-awards/google-academic-research-award-program-recipients/`

[3] `https://research.facebook.com/blog/`

our estimate of overall funding influence is a floor, not a ceiling. Moreover, it is unclear how many gifts were given from companies not through publicly disclosed RFPs. Table S1 displays the number of unique authors and unique author-company-year combinations for each of our three categories of disclosable interests.

For editors, it was tractable to supplement our identification with manual review of each of their CVs or personal websites, when available. From each editor's CV, we identified indications of funding from each of our four firms. We did not extract collaboration or prior employment, and leveraged our general approach to identify these ties among editors.

### S2.1 Conservative approach to estimation

Our goal throughout is to anchor our analysis in ties that can be identified with a high degree of certainty. Additionally, our reliance on public data inherently limits our ability to detect ties to industry. Below we provided a short list of ways in which either the constrains of our design or our design choices were intended to produce a conservative estimate.

- Employment
  - Identified employment solely through publication with affiliation, excluding non-publishing employees.
  - We did not assume continued employment between years in which authors published while affiliated with industry.
  - Manually verified employment of those remaining.
- Funding
  - We relied on conservative assumptions regarding funding duration.
  - We were unable to obtain data on RFPs from Microsoft and X, limiting our detection of funding.
  - We were unable to identify any funding not disclosed through the remaining firm's announcements.
  - For funding identified through the literature, we manually verified the recipients.
  - As it was tractable, we manually verified funding using CVs for reviewers and editors.

  - We did not "double count" employment as funding, even though companies provide resources for employees.
  - We also did not not "double count" resources provided during collaboration as funding.
  - We additionally excluded megastudies, which may have lead to inflated numbers of authors tied to industry.
  - We chose not to include funding from charities run by individuals or organizations with close ties to social media firms.

- Collaboration
  - We assumed a conservative duration for collaborations, except in the case of the 2020 US election collaboration with Meta for which the start date is a matter of public record.
  - We limited collaboration to those matching search terms related to social media, ignoring collaboration that may have been about other topics.
  - We did not attempt to identify informal roles, such as membership on advisory boards.

- Misc.
  - We limited our analysis to scientific articles, excluding other forms of scientific communication.
  - We estimated independence in peer review with just two reviewers, as three or more would lead to higher estimates of saturation.
  - We used weakly informative priors throughout the analysis and simple statistical models to avoid analytic choices influencing results.

## S3 Analysis

Our analysis largely links detected disclosable ties to the literature, authors and editors. Our intent in doing so is to provide a description of the rates at which disclosable ties occur, the patterns of industry investment in authors, relative impact of papers, and some trends over time. We note that each of these are purely descriptive, and not meant to test any specific hypothesis. We use statistical models throughout to quantify our descriptive uncertainty,

but do not leverage them to develop evidence for or against any specific model (e.g., a null).

We present 95% credible regions throughout, but note that discerning whether they include or exclude any given parameter (say, zero) is not a goal of our analyses. Indeed, the choice of 95% is arbitrary to ensure broad coverage of uncertainty and ease understanding for readers unfamiliar with Bayesian models. The primary reason for leveraging description rather than hypothesis testing is that there are no coherent nulls to be found in our empirical questions.

For example, there is no anticipated null rate at which papers would have ties to industry—we know *a priori* it is not 0%, nor is it 100%. Similarly, with trends over time there is no reason to believe that norms surrounding disclosure will remain static. An alternative to hypothesis testing would be evaluating the plausibility of competing (perhaps causal) models, however we do not examine causality here as we lack data to ask even basic causal questions, such as the motivating factors for failing to disclose a tie to industry.

## S3.1 Literature

For each paper in our corpus we began by checking whether any author was employed by the company, resulting in a binary variable indicating industry (co-)authorship. This was repeated for the manually annotated rates of competing interests disclosure (Disclosed), as well as the rates at which company ties could be identified elsewhere in the paper (Identifiable). Next, for each paper we examined whether any disclosable interest existed in our dataset, for any author, within each respective journal's policy for recency. The resultant binary vector provided our estimate of "found" reported in the main text. Finally, we categorized any papers for which any of the above vectors were true has having "any" disclosable tie. For each, we calculated the percentage and associated credible region using Bayesian binomial estimation (See S3.5.1). To evaluate norms over time, we leveraged a Bayesian binomial regression, as described in S3.5.2.

We then noted for each paper the distinct types of competing interests that arose from authors: Employment, Collaboration or Funding. Here too, we constructed binary vectors and estimated the percentage of each type, as well as their associated credible regions, using Bayesian Binomial estimation. Next, we gathered data from Altmetrics using the DOI for each paper provided by OpenAlex. For simplicity and to minimize our assumptions made, we simply used an empirical Bayesian Negative Binomial

regression with a single predictor indicating the presence of a tie to industry (See Section S3.5.3).

## S3.2 Authors

Our author analysis is similar our analysis of literature, however we map the presence of disclosable ties to authors alone. We begin by simply calculating the proportion of authors with a tie to industry, quantifying our uncertainty using binomial estimation as elsewhere (See Sec. S3.5.1). This is repeated based to evaluate other questions, such as the nature of the tie or the company to which authors are tied.

We then calculate the total industry engagement for each author by simplifying our data-frame to columns for author, company, year, and type and de-duplicating. This results in a count of the number of years in which a given author received support, of a given form, from a given company. For example, 3 years of funding with Meta alongside 2 years of collaboration with Microsoft would yield 5 years—even if those years overlapped. We used this distribution across authors to calculate the Gini coefficient and produce the curve seen in the main text. We estimate average company years using Bayesian methods for a Negative Binomial Distribution (See Sec. S3.5.4)

We also use this per-author measure as a predictor in a Bayesian Binomial regression to estimate whether authors with more support from industry are more likely to disclose those ties (See Sec. S3.5.5). We estimate the marginal change over ten years of industry funding, reported in the paper, by subtracting the posterior predictive distribution calculated at ten years from the value at one year. Finally, for each author we count the number of papers they are associated with in our corpus, and use that as input to a logistic regression with the probability of any disclosable tie as a predictor (See Sec. S3.5.6)

## S3.3 Editors and Reviewers

We began by manual review of editor's CVs, noting years in which they received funding from or were employed by technology companies. We then matched editors to their OpenAlex IDs, and performed our usual check of disclosable interests described above. This produced a dataset for each editor of the years in which they were funded, employed, or collaborated with industry. We characterized the percent of editors as with authors using Binomial estimation (See Sec. S3.5.1). We then repeated the process for papers

edited, using Multinational estimation to account for the combinatorial possibilities of authors and editors having competing interests (SI Sec. S3.6). We leveraged the same approach to identify reviewer disclosable interests.

### S3.4 Topical Bias

To evaluate topical bias, we constructed the bibliographic coupling network defining and edge weight between two papers ($w_{ij}$) as:

$$w_{ij} = \frac{|r_i \cap r_j|}{\sqrt{|r_i| \cdot |r_j|}}$$

where:

$$|r_i \cap r_j| = \text{count of shared references between paper } i \text{ and paper } j$$
$$|r_i|, |r_j| = \text{count of references for paper } i \text{ and paper } j \text{ respectively}$$

From there we kept the $K = 4$ K-Truss, as in our identification of the core corpus. Next, we applied Louvain community detection in NetworkX using a resolution of 1.0, a threshold of 0.0, and a random seed of 42 (used for all seeds) [2]. This yielded our five communities. Taking the count of industry-tied paper in each community, we estimated their proportion and associated uncertainty using hierarchical Binomial estimation (See S3.6.1).

To identify topics, we took the abstracts from each paper and removed english stop words using Scikit-learn [3]. We also included "abstract", "social", and "media". For supervised topic learning, we used BERTopic [4]. Our custom stopwords were fed into CountVectorizer, with $n$-grams up to trigrams. We additionally used a class-based Term Frequency-Inverse Document Frequency transformer to generate distinguishing words associated with each topic.

Given the somewhat opaque nature of BERTopic, we supplemented this approach with a more traditional NLP analysis. Our goal was to use the simplest analysis possible, as a point of comparison to evaluate robustness. We restricted this analysis to the two communities which differed in abundance of industry-connected research. We lemmatized abstracts, removing non-alphabetic characters and the same stopwords as above. We used sci-kit learn's TfidfVectorizer with up to trigrams for each of the two communities. We subtracted the feature vectors and identified top terms that differed in

frequency most across the two communities. Results can be seen in figure S4.

Finally, for estimating impact we relied on the same model as used for the literature (SI Sec. S3.5.3). Outcomes are listed as tables below (SI Table S22-S27). Posterior predictive distributions are shown in figure S8.

## S3.5 Statistical Models

All models were fit using the No-U-Turn-Sampler (NUTS) in PYMC 5.25.1 [5]. We used 2000 tuning steps, and 2000 draws for four chains, with "adapt delta" set to .95, leaving all remaining arguments as defaults unless otherwise noted. We ensured that $\hat{r} \approx 1.0$ for all critical parameters and checked for sufficient samples to support inference in the ESS Bulk and Tail, which are reported below. Additional model-specific validation is noted where relevant in the model descriptions.

### S3.5.1 Binomial Estimation

Many of our figures involves assignment of a credible region given a binomially distributed variable, such as the number of papers with disclosable interests out of all papers. We use the simplest possible model to estimate the probability, $\theta$:

$$\begin{aligned} \theta &\sim \text{Beta}(2, 2) \\ K &\sim \text{Binomial}(N,\ \theta) \end{aligned}$$

Here, $N$ and $K$ are set by data. We use the same weakly informative, generic Beta prior for all estimation of binomial data, unless otherwise indicated.

### S3.5.2 Norms Over Time

To model norms over time, we used a binomial regression with a logit link function such that:

$$\alpha \sim \text{Normal}(0, 1)$$
$$\beta \sim \text{Normal}(0, 1)$$
$$\text{logit}(p_i) = \alpha + \beta\, t_{c,i}$$
$$y_i \sim \text{Binomial}(N_i,\, p_i)\,,$$

Where $i$ indicates the observation across years, $t_c$ is time (in years, centered), $N_i$ is the number of disclosed papers in a given year out of out of $K_i$. We used weakly informative, generic priors for the intercept ($\alpha$) and the effect of time $\beta$. There were no divergent transitions, and the posterior predictive fit visually conformed with the raw rates, as seen in the main text figure. A table of relevant coefficients can be found below (Table S6).

### S3.5.3 Paper Impact

To model paper impact, we use a negative Binomial regression. We use weakly informative generic priors, allowing us to apply the same model to each metric and avoid bespoke priors on any given metric. One exception is the hyper-prior for $\beta_0$, which we construct as an empirical prior using the mean across all of the data for a given metric. Specifically our model of impact is:

$$\begin{aligned}
\beta_0 &\sim \text{Normal}(\mu_a, 1) \\
\beta_1 &\sim \text{Normal}(0,\, 1), \\
\log(\mu_i) &= \beta_0 + \beta_1 x_i \\
\alpha_j &\sim \text{LogNormal}(\text{Log}(50), 0.75) \quad j \in \{0, 1\} \\
y_i &\sim \text{NegBinom}(\mu_i,\ \alpha_{x_i})\,,
\end{aligned}$$

Where $\beta_0$ is the average impact of a given article and $\beta_1$ is the effect of industry ties. The over-dispersion parameter, $\alpha$ is set generically and allowed to be distinct for each of the two classes of articles. With this model formulation, the relative impact is simply: $\exp(\beta_1)$. We validate this model using posterior predictive distributions across all metrics, and ensuring reasonable visual fit (Fig. S6). We additionally show the actual relative mean impact overlaid with the posterior predictive means and 95% Credible Region (Fig. S7). There were no divergent transitions and other sampling summary statistics can be found in tables S7-S13.

### S3.5.4 Negative Binomial Estimation

To estimate years of support we leverage a negative binomial distribution, parameterized as the mean ($\mu$) and shape parameter $\alpha$:

$$\mu \sim \text{HalfNormal}(0, 5) \tag{S1}$$
$$\phi \sim \text{Exponential}(1) \tag{S2}$$
$$y_i \sim \text{NegBinomial}(\mu, \alpha) \tag{S3}$$

We use generic, weakly informative priors for each parameter. There were no divergent transitions and other sampling summary statistics can be found in Table S16. A posterior predictive distribution can be seen in Figure S5.

### S3.5.5 Binomial Author Norm Regression

Our logistic regression to estimate author disclosure rates with increasing ties to industry is straightforward in form and nearly identical to our model of norms over time in Sec. S3.5.2, differing only in notation:

$$\begin{aligned}
\alpha &\sim \text{Normal}(0, 1) \\
\beta &\sim \text{Normal}(0, 1) \\
\text{logit}(p_i) &= \alpha + \beta\, x_i \\
K_i &\sim \text{Binomial}(N_i,\, p_i)\,,
\end{aligned}$$

We use generic, weakly informative priors for $\alpha$ and $\beta$. The sole predictor, $x_i$, indicates the standardized years of support for the $i^{th}$ author. $N_i$ is the number of papers in our corpus which, for a given author met a journal's criteria for disclosing a competing interest. $K_i$ is the number of papers for which that author affirmatively declared competing interests. There were no divergent transitions and other sampling summary statistics can be found in Table S17.

### S3.5.6 Paper Count Logistic Regression

Our logistic regression for any disclosable interest tie as a function of papers in corpus is straightforward:

$$\begin{aligned}
\alpha &\sim \text{Normal}(0, 1) \\
\beta &\sim \text{Normal}(0, 1) \\
\text{logit}(p_i) &= \alpha + \beta\, x_i \\
Y_i &\sim \text{Bernoulli}(p_i)\,,
\end{aligned}$$

Here, $x_i$ is the number of papers in corpus. Generic, weakly informative priors are used for $\alpha$ and $\beta$. Presence or absence of disclosable ties is indicated by $Y_i$. There were no divergent transitions and sampling summary statistics can be found in table S18.

## S3.6 Multinomial Estimation

Some of our outcomes are multinomial, such as whether Editors, Authors, Neither or Both are tied to industry. The probability of these categories must sum to one, so we rely on Multinomial estimation with a Dirichlet prior. The Dirichlet distribution can be viewed as a multi-dimensional extension of a Beta distribution and is a natural choice for a Multinomial outcome. We use Jeffrey's prior as more informative distributions might push mass towards an equiprobable distribution. This choice of prior also captures the fact that for the contexts in which we used this, we had truly no idea what to expect.

$$\begin{aligned}
&p = (p_1, \ldots, p_K) \\
&p \sim \text{Dirichlet}\big(\tfrac{1}{2},\, \ldots,\, \tfrac{1}{2}\big) \\
&y \sim \text{Multinomial}(n,\, p)\,,
\end{aligned}$$

Here $p$ is the probability for a given outcome out of $k$ outcomes (four in the example above). The number of papers in each class $y$, is estimated using $p$ and the total number of papers ($n$).

### S3.6.1 Hierarchical Binomial Estimation

To estimate the abundance of industry-tied papers in each field, we leveraged a hierarchical binomial estimation. Specifically:

$$\alpha \sim \text{Normal}(0, 1) \tag{S4}$$

$$\beta_i \sim \text{Normal}(\alpha, 1) \quad i \in \{0, ..., 5\} \tag{S5}$$

$$\text{logit}(p_i) = \beta_i \tag{S6}$$

$$Y_j \sim \text{Binomial}(p_i, N_j)\,, \tag{S7}$$

Here, $\alpha$ represents the overall average proportion of papers with ties to industry, and $\beta$ characterizes the deviation from that average per topic. $N_J$ is the number of papers per topic, and $K_j$ is the number of papers with disclosable ties.

## S4 Supplemental Tables

| Type | Unique Authors | Author-Year-Company |
|---|---|---|
| Employment | 60 | 460 |
| Funding | 97 | 299 |
| Collaboration | 193 | 891 |

Table S1: Counts of disclosable interests identified by unique authors per type, as well as the unique author/company/year combinations.

| y | N | K | Mean | 5% | 95% |
|---|---|---|---|---|---|
| Industry | 295 | 23 | 8.1 | 5.2 | 11.6 |
| Disclosed | 295 | 38 | 13.1 | 9.5 | 17.2 |
| Identifiable | 295 | 58 | 19.9 | 15.5 | 24.6 |
| Found | 295 | 146 | 49.4 | 43.5 | 55.3 |
| Any | 295 | 149 | 50.5 | 44.9 | 56.2 |

Table S2: Identifiability of disclosable interests in published papers. Employment indicates the proportion of papers with industry affiliations among the authorship. Disclosed indicates the rate at which industry ties are indicated in competing interests statements. Identifiable is the proportion for which disclosable interests can be found by reading the pdf, although not necessarily in a competing interests statement. Found indicates the proportion for which we identified a disclosable interest and any indicates any one of the previous categories.

| y | N | K | Mean | 5% | 95% |
|---|---|---|---|---|---|
| Employment | 295 | 43 | 14.9 | 10.9 | 19.3 |
| Funding | 295 | 78 | 26.6 | 21.8 | 31.7 |
| Multiple | 295 | 79 | 26.9 | 22.0 | 32.2 |
| Collaboration | 295 | 128 | 43.4 | 37.8 | 49.1 |

Table S3: Types of disclosable interests associated with published papers, among papers with at least one disclosable interest. Collaboration, employment, and funding are as described above and must have occured within the relevant journal's time frame for disclosure. Multiple indicates that a paper had multiple types of disclosable interests, among or across authors

| y | N | K | Mean | 5% | 95% |
|---|---|---|---|---|---|
| Disclosed | 227 | 0 | 0.4 | 0.0 | 1.5 |
| Industry | 227 | 5 | 2.6 | 1.0 | 5.1 |
| Identifiable | 227 | 15 | 6.9 | 4.0 | 10.6 |
| Found | 227 | 96 | 42.4 | 36.2 | 48.8 |
| Any | 227 | 97 | 42.8 | 36.3 | 49.2 |

Table S4: As in table S2, however subset to the 229 papers which affirmatively declared no competing interest.

| y | N | K | Mean | 5% | 95% |
|---|---|---|---|---|---|
| Employment | 295 | 43 | 14.9 | 10.9 | 19.3 |
| Funding | 295 | 78 | 26.6 | 21.8 | 31.7 |
| Multiple | 295 | 79 | 26.9 | 22.0 | 32.2 |
| Collaboration | 295 | 128 | 43.4 | 37.8 | 49.1 |

Table S5: Types of disclosable interests for each paper.

| Param | Mean | sd | 5% | 95% | MCSE | MCSE SD | ESS Bulk | ESS Tail | $\hat{r}$ |
|---|---|---|---|---|---|---|---|---|---|
| alpha | -1.08 | 0.28 | -1.67 | -0.56 | 0.01 | 0.00 | 2658.98 | 3367.36 | 1.00 |
| beta | 0.01 | 0.06 | -0.11 | 0.13 | 0.00 | 0.00 | 2498.85 | 3056.59 | 1.00 |

Table S6: Regression coefficients for the Bayesian binomial regression of the rate at which disclosable interests are evidenced as competing interests over time.

| DI | Attention | News | Citations | Policy | Social Media | Wikipedia |
|---|---|---|---|---|---|---|
| None | 401.49 | 39.18 | 138.48 | 1.72 | 246.10 | 1.03 |
| Found | 644.34 | 67.03 | 220.82 | 3.32 | 435.79 | 1.79 |

Table S7: Average impact disaggregated papers with and without an identified disclosable interest. Each metric is as calculated by Altmetrics with the exception of Social Media Mentions. For that, we take the sum across several platforms: Weibo, Google+, Facebook, X, Bluesky, Videos (e.g. Youtube), Reddit, Pinterest, and LinkedIn

| Param | Mean | sd | 5% | 95% | MCSE | MCSE SD | ESS Bulk | ESS Tail | $\hat{r}$ |
|---|---|---|---|---|---|---|---|---|---|
| $\beta_0$ | 6.01 | 0.11 | 5.80 | 6.23 | 0.00 | 0.00 | 4555.70 | 4847.45 | 1.00 |
| $\beta_1$ | 0.46 | 0.15 | 0.17 | 0.78 | 0.00 | 0.00 | 4656.16 | 5149.44 | 1.00 |
| $\alpha_0$ | 0.56 | 0.05 | 0.46 | 0.67 | 0.00 | 0.00 | 7025.18 | 5366.67 | 1.00 |
| $\alpha_1$ | 0.55 | 0.05 | 0.45 | 0.65 | 0.00 | 0.00 | 7563.11 | 5817.40 | 1.00 |

Table S8: Sampling summary for News impact model

| Param | Mean | sd | 5% | 95% | MCSE | MCSE SD | ESS Bulk | ESS Tail | $\hat{r}$ |
|---|---|---|---|---|---|---|---|---|---|
| $\beta_0$ | 3.69 | 0.14 | 3.43 | 3.95 | 0.00 | 0.00 | 4569.25 | 5737.42 | 1.00 |
| $\beta_1$ | 0.51 | 0.19 | 0.14 | 0.90 | 0.00 | 0.00 | 4503.23 | 5651.88 | 1.00 |
| $\alpha_0$ | 0.38 | 0.04 | 0.30 | 0.46 | 0.00 | 0.00 | 7299.90 | 5446.53 | 1.00 |
| $\alpha_1$ | 0.35 | 0.03 | 0.29 | 0.42 | 0.00 | 0.00 | 6753.34 | 4990.31 | 1.00 |

Table S9: Sampling summary for News impact model

| Param | Mean | sd | 5% | 95% | MCSE | MCSE SD | ESS Bulk | ESS Tail | $\hat{r}$ |
|---|---|---|---|---|---|---|---|---|---|
| $\beta_0$ | 4.95 | 0.12 | 4.72 | 5.18 | 0.00 | 0.00 | 5596.29 | 5475.32 | 1.00 |
| $\beta_1$ | 0.45 | 0.19 | 0.11 | 0.83 | 0.00 | 0.00 | 5473.57 | 5725.33 | 1.00 |
| $\alpha_0$ | 0.51 | 0.05 | 0.41 | 0.61 | 0.00 | 0.00 | 8203.37 | 5815.02 | 1.00 |
| $\alpha_1$ | 0.33 | 0.03 | 0.26 | 0.39 | 0.00 | 0.00 | 8170.12 | 5612.47 | 1.00 |

Table S10: Sampling summary for Citations impact model

| Param | Mean | sd | 5% | 95% | MCSE | MCSE SD | ESS Bulk | ESS Tail | $\hat{r}$ |
|---|---|---|---|---|---|---|---|---|---|
| $\beta_0$ | 0.58 | 0.17 | 0.25 | 0.91 | 0.00 | 0.00 | 4385.07 | 4579.37 | 1.00 |
| $\beta_1$ | 0.61 | 0.25 | 0.11 | 1.10 | 0.00 | 0.00 | 4501.07 | 4652.99 | 1.00 |
| $\alpha_0$ | 0.28 | 0.05 | 0.18 | 0.37 | 0.00 | 0.00 | 7498.88 | 5288.99 | 1.00 |
| $\alpha_1$ | 0.19 | 0.03 | 0.14 | 0.25 | 0.00 | 0.00 | 7152.75 | 5521.87 | 1.00 |

Table S11: Sampling summary for Policy impact model

| Param | Mean | sd | 5% | 95% | MCSE | MCSE SD | ESS Bulk | ESS Tail | $\hat{r}$ |
|---|---|---|---|---|---|---|---|---|---|
| $\beta_0$ | 5.52 | 0.11 | 5.31 | 5.74 | 0.00 | 0.00 | 4719.24 | 4974.56 | 1.00 |
| $\beta_1$ | 0.55 | 0.16 | 0.23 | 0.85 | 0.00 | 0.00 | 4627.03 | 5059.08 | 1.00 |
| $\alpha_0$ | 0.55 | 0.05 | 0.44 | 0.65 | 0.00 | 0.00 | 7222.96 | 5355.88 | 1.00 |
| $\alpha_1$ | 0.50 | 0.05 | 0.41 | 0.59 | 0.00 | 0.00 | 7195.53 | 5415.80 | 1.00 |

Table S12: Sampling summary for Social Media impact model

| Param | Mean | sd | 5% | 95% | MCSE | MCSE SD | ESS Bulk | ESS Tail | $\hat{r}$ |
|---|---|---|---|---|---|---|---|---|---|
| $\beta_0$ | 0.07 | 0.19 | -0.31 | 0.44 | 0.00 | 0.00 | 5597.85 | 5275.71 | 1.00 |
| $\beta_1$ | 0.50 | 0.28 | -0.05 | 1.03 | 0.00 | 0.00 | 5584.41 | 5723.78 | 1.00 |
| $\alpha_0$ | 0.24 | 0.05 | 0.15 | 0.35 | 0.00 | 0.00 | 7024.90 | 5003.22 | 1.00 |
| $\alpha_1$ | 0.16 | 0.03 | 0.11 | 0.22 | 0.00 | 0.00 | 7188.81 | 5134.82 | 1.00 |

Table S13: Sampling summary for Wikipedia impact model

| y | N | K | Mean | 5% | 95% |
|---|---|---|---|---|---|
| Employment | 1210 | 60 | 5.0 | 3.8 | 6.3 |
| Multiple | 1210 | 83 | 7.0 | 5.6 | 8.5 |
| Funding | 1210 | 90 | 7.5 | 6.1 | 9.1 |
| Collaboration | 1210 | 199 | 16.5 | 14.5 | 18.7 |
| Any | 1210 | 255 | 21.2 | 18.9 | 23.5 |

Table S14: Identifiability of disclosable interests among authors. Employment indicates the proportion of papers with industry affiliations among the authorship. Disclosed indicates the rate at which industry ties are indicated in competing interests statements. Identifiable is the proportion for which disclosable interests can be found by reading the pdf, although not necessarily in a competing interests statement. Found indicates the proportion for which we identified a disclosable interest and any indicates any one of the previous categories.

| y | N | K | Mean | 5% | 95% |
|---|---|---|---|---|---|
| Twitter | 1210 | 10 | 0.9 | 0.5 | 1.5 |
| Microsoft | 1210 | 72 | 6.0 | 4.7 | 7.4 |
| Multiple | 1210 | 83 | 7.0 | 5.6 | 8.5 |
| Google | 1210 | 98 | 8.2 | 6.7 | 9.8 |
| Meta | 1210 | 163 | 13.5 | 11.7 | 15.5 |

Table S15: Among authors with competing interests, the percentage that engaged with each of the four firms or multiple firms.

| Param | Mean | sd | 5% | 95% | MCSE | MCSE SD | ESS Bulk | ESS Tail | $\hat{r}$ |
|---|---|---|---|---|---|---|---|---|---|
| mu | 1.27 | 0.13 | 1.04 | 1.54 | 0.00 | 0.00 | 4119.00 | 2889.00 | 1.00 |
| alpha | 0.09 | 0.01 | 0.08 | 0.11 | 0.00 | 0.00 | 4264.00 | 2734.00 | 1.00 |

Table S16: Parameters for our estimate of company-years of industry support

| Param | Mean | sd | 5% | 95% | MCSE | MCSE SD | ESS Bulk | ESS Tail | $\hat{r}$ |
|---|---|---|---|---|---|---|---|---|---|
| alpha | 0.23 | 0.09 | 0.05 | 0.40 | 0.00 | 0.00 | 3870.00 | 2891.00 | 1.00 |
| beta | 0.16 | 0.10 | -0.04 | 0.35 | 0.00 | 0.00 | 3585.00 | 3045.00 | 1.00 |

Table S17: Regression coefficients for the Bayesian binomial regression of the rate at which authors disclose competing interests as a function of the extent of their ties to industry.

| Param | Mean | sd | 5% | 95% | MCSE | MCSE SD | ESS Bulk | ESS Tail | $\hat{r}$ |
|---|---|---|---|---|---|---|---|---|---|
| alpha | -2.37 | 0.14 | -2.63 | -2.10 | 0.00 | 0.00 | 2135.00 | 2556.00 | 1.00 |
| beta | 0.71 | 0.08 | 0.56 | 0.87 | 0.00 | 0.00 | 1997.00 | 2610.00 | 1.00 |

Table S18: Regression coefficients for the Bayesian logistic regression of the probability that authors possess a tie to industry as a function of the number of papers they published in the corpus.

| Param | Mean | sd | 5% | 95% | MCSE | MCSE SD | ESS Bulk | ESS Tail | $\hat{r}$ |
|---|---|---|---|---|---|---|---|---|---|
| alpha | -1.58 | 0.36 | -2.29 | -0.89 | 0.01 | 0.01 | 2662.00 | 3292.00 | 1.00 |
| beta | 0.31 | 0.13 | 0.07 | 0.56 | 0.00 | 0.00 | 2846.00 | 3356.00 | 1.00 |

Table S19: Regression coefficients for the Bayesian logistic regression of the probability that editors possess a tie to industry as a function of the number of papers they edited in the corpus.

| Name | Publications | Representation |
|---|---|---|
| Political Behavior | 79 | political, polarization, users, content, speech, moral, online, partisan, group, hate |
| Mental Health | 63 | depression, language, health, use, data, change, based, people, level, self |
| Social Networks | 60 | misinformation, news, false, information, sharing, political, fact, quality, online, users |
| Misinfo Sharing | 57 | ties, networks, data, information, high, network, online, economic, individual, ses |
| Platform Dynamics | 33 | users, communities, news, dynamics, antivaccine, activity, platforms, content, network, fake |

Table S20: Communities identified, the number of publications, and words associated with that community

| Community | Mean | sd | 5% | 95% | MCSE | MCSE SD | ESS Bulk | ESS Tail | $\hat{r}$ |
|---|---|---|---|---|---|---|---|---|---|
| Social Network Analysis | 0.71 | 0.06 | 0.61 | 0.83 | 0.00 | 0.00 | 1288.00 | 756.00 | 1.00 |
| Misinfo Sharing | 0.52 | 0.06 | 0.40 | 0.63 | 0.00 | 0.00 | 1314.00 | 689.00 | 1.00 |
| Platform dynamics | 0.24 | 0.07 | 0.11 | 0.37 | 0.00 | 0.00 | 1006.00 | 552.00 | 1.01 |
| Mental Health | 0.43 | 0.06 | 0.31 | 0.53 | 0.00 | 0.00 | 1329.00 | 673.00 | 1.00 |
| Political Behavior | 0.52 | 0.06 | 0.40 | 0.63 | 0.00 | 0.00 | 1454.00 | 604.00 | 1.00 |

Table S21: Probability of disclosable ties across the five communities, alongside model output

| Param | Mean | sd | 5% | 95% | MCSE | MCSE SD | ESS Bulk | ESS Tail | $\hat{r}$ |
|---|---|---|---|---|---|---|---|---|---|
| $\beta_0$ | 6.25 | 0.23 | 5.81 | 6.72 | 0.00 | 0.00 | 4661.92 | 4676.20 | 1.00 |
| $\beta_1$ | 0.14 | 0.28 | -0.43 | 0.65 | 0.00 | 0.00 | 4545.96 | 4840.16 | 1.00 |
| $\alpha_0$ | 0.57 | 0.10 | 0.37 | 0.78 | 0.00 | 0.00 | 5771.09 | 4547.40 | 1.00 |
| $\alpha_1$ | 0.80 | 0.12 | 0.56 | 1.02 | 0.00 | 0.00 | 6125.17 | 4679.27 | 1.00 |

Table S22: Sampling summary for overall ALtmetric impact model across communities associated with industry (misinformation sharing) or independence (platform dynamics)

| Param | Mean | sd | 5% | 95% | MCSE | MCSE SD | ESS Bulk | ESS Tail | $\hat{r}$ |
|---|---|---|---|---|---|---|---|---|---|
| $\beta_0$ | 4.11 | 0.27 | 3.59 | 4.66 | 0.00 | 0.00 | 3367.67 | 3624.56 | 1.00 |
| $\beta_1$ | -0.06 | 0.33 | -0.71 | 0.59 | 0.01 | 0.00 | 3356.55 | 4068.73 | 1.00 |
| $\alpha_0$ | 0.40 | 0.08 | 0.25 | 0.56 | 0.00 | 0.00 | 6628.83 | 4778.26 | 1.00 |
| $\alpha_1$ | 0.48 | 0.08 | 0.34 | 0.63 | 0.00 | 0.00 | 6465.34 | 4999.84 | 1.00 |

Table S23: Sampling summary for News impact model across communities associated with industry (misinformation sharing) or independence (platform dynamics)

| Param | Mean | sd | 5% | 95% | MCSE | MCSE SD | ESS Bulk | ESS Tail | $\hat{r}$ |
|---|---|---|---|---|---|---|---|---|---|
| $\beta_0$ | 4.95 | 0.12 | 4.72 | 5.18 | 0.00 | 0.00 | 5596.29 | 5475.32 | 1.00 |
| $\beta_1$ | 0.45 | 0.19 | 0.11 | 0.83 | 0.00 | 0.00 | 5473.57 | 5725.33 | 1.00 |
| $\alpha_0$ | 0.51 | 0.05 | 0.41 | 0.61 | 0.00 | 0.00 | 8203.37 | 5815.02 | 1.00 |
| $\alpha_1$ | 0.33 | 0.03 | 0.26 | 0.39 | 0.00 | 0.00 | 8170.12 | 5612.47 | 1.00 |

Table S24: Sampling summary for Citations impact model across communities associated with industry (misinformation sharing) or independence (platform dynamics)

| Param | Mean | sd | 5% | 95% | MCSE | MCSE SD | ESS Bulk | ESS Tail | $\hat{r}$ |
|---|---|---|---|---|---|---|---|---|---|
| $\beta_0$ | 0.97 | 0.32 | 0.32 | 1.60 | 0.00 | 0.00 | 4439.31 | 4005.59 | 1.00 |
| $\beta_1$ | -0.04 | 0.40 | -0.86 | 0.72 | 0.01 | 0.00 | 4412.02 | 4231.58 | 1.00 |
| $\alpha_0$ | 0.32 | 0.10 | 0.14 | 0.51 | 0.00 | 0.00 | 5963.94 | 4951.28 | 1.00 |
| $\alpha_1$ | 0.28 | 0.07 | 0.16 | 0.42 | 0.00 | 0.00 | 6196.24 | 4806.20 | 1.00 |

Table S25: Sampling summary for Policy impact model across communities associated with industry (misinformation sharing) or independence (platform dynamics)

| Param | Mean | sd | 5% | 95% | MCSE | MCSE SD | ESS Bulk | ESS Tail | $\hat{r}$ |
|---|---|---|---|---|---|---|---|---|---|
| $\beta_0$ | 5.55 | 0.23 | 5.12 | 6.02 | 0.00 | 0.00 | 3123.56 | 2884.22 | 1.00 |
| $\beta_1$ | 0.49 | 0.28 | -0.04 | 1.05 | 0.01 | 0.00 | 3026.93 | 3137.81 | 1.00 |
| $\alpha_0$ | 0.61 | 0.11 | 0.40 | 0.83 | 0.00 | 0.00 | 5650.03 | 4585.57 | 1.00 |
| $\alpha_1$ | 0.67 | 0.10 | 0.49 | 0.87 | 0.00 | 0.00 | 6080.48 | 5077.10 | 1.00 |

Table S26: Sampling summary for Social Media impact model across communities associated with industry (misinformation sharing) or independence (platform dynamics)

| Param | Mean | sd | 5% | 95% | MCSE | MCSE SD | ESS Bulk | ESS Tail | $\hat{r}$ |
|---|---|---|---|---|---|---|---|---|---|
| $\beta_0$ | 0.24 | 0.20 | -0.15 | 0.64 | 0.00 | 0.00 | 5891.25 | 5204.85 | 1.00 |
| $\beta_1$ | 0.26 | 0.38 | -0.43 | 1.03 | 0.00 | 0.00 | 5696.83 | 5503.57 | 1.00 |
| $\alpha_0$ | 0.68 | 0.24 | 0.30 | 1.18 | 0.00 | 0.00 | 7827.65 | 5120.31 | 1.00 |
| $\alpha_1$ | 0.39 | 0.14 | 0.16 | 0.66 | 0.00 | 0.00 | 8638.59 | 5937.65 | 1.00 |

Table S27: Sampling summary for Wikipedia impact model across communities associated with industry (misinformation sharing) or independence (platform dynamics)

| Topic | Attention | News | Citations | Policy | Social Media | Wikipedia |
|---|---|---|---|---|---|---|
| Misinfo Sharing | 592.66 | 56.29 | 119.31 | 2.45 | 421.93 | 1.24 |
| Network Dynamics | 499.13 | 59.74 | 242.94 | 2.55 | 240.13 | 1.65 |

Table S28: Average impact disaggregated papers across the two topics which differed in industry ties. Each metric is reported as calculated by Altmetrics with the exception of Social Media Mentions. For that, we take the sum across several platforms: Weibo, Google+, Facebook, X, Bluesky, Videos (e.g. Youtube), Reddit, Pinterest, and LinkedIn

| Topic | Attention | News | Citations | Policy | Social Media | Wikipedia |
|---|---|---|---|---|---|---|
| Misinfo Sharing | 34374.00 | 3265.00 | 6920.00 | 142.00 | 24894.00 | 72.00 |
| Network Dynamics | 15473.00 | 1852.00 | 7531.00 | 79.00 | 7444.00 | 51.00 |

Table S29: Total impact across the two topics which differed in industry ties. Each metric is reported as calculated by Altmetrics with the exception of Social Media Mentions. For that, we take the sum across several platforms: Weibo, Google+, Facebook, X, Bluesky, Videos (e.g. Youtube), Reddit, Pinterest, and LinkedIn

## S5 Supplemental Figures

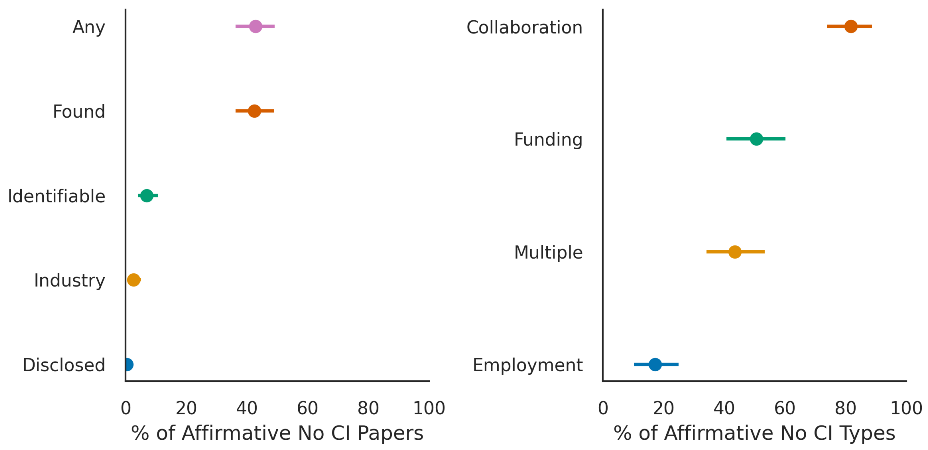


Figure S1: Subset analysis among published work which affirmatively declares no competing interests **A)**Disclosable interests that were either indicated by affiliation (Industry), indicated by in competing interest statements (disclosed), found elsewhere in the manuscript (Identifiable), found through our broader search (found), or any combination of the above (Any). **B)** Percentage of papers containing at least one of a given type of disclosable interest.

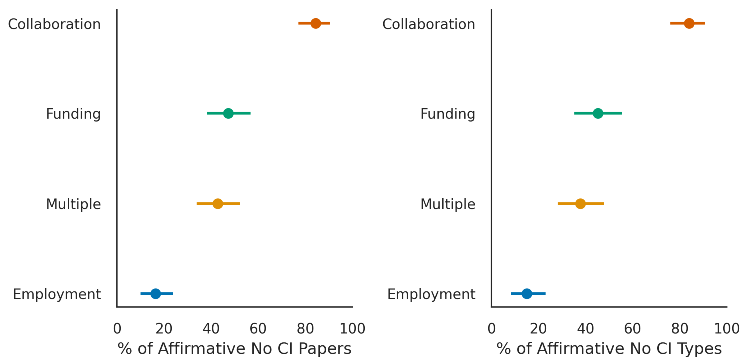


Figure S2: **A)** Disclosable interest by type among papers lacking competing interests disclosures **B)** Disclosable interest by type among papers for which no ties to industry can be discerned anywhere in the manuscript.

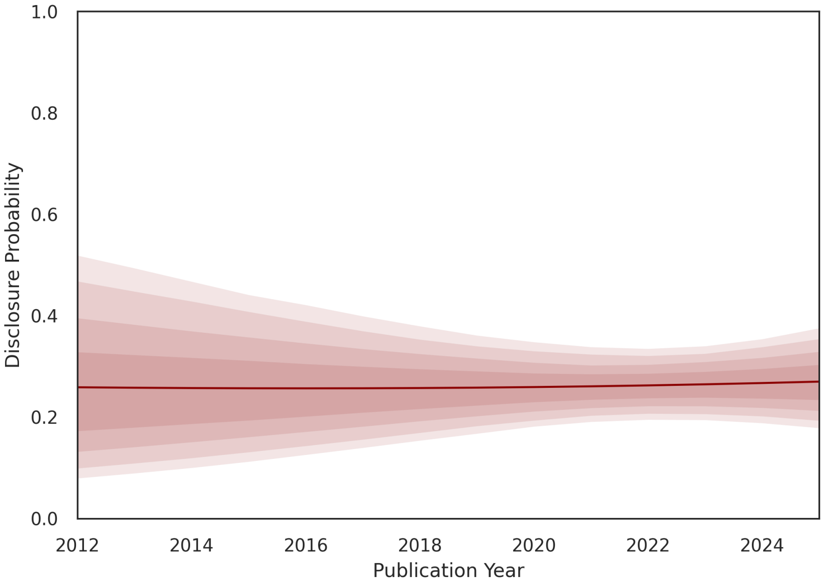


Figure S3: Bayesian Binomial Regression of the probability that a published paper with a disclosable interest lists it as a competing interests. Shaded bands correspond to 50, 75, 89, 95% credible regions.

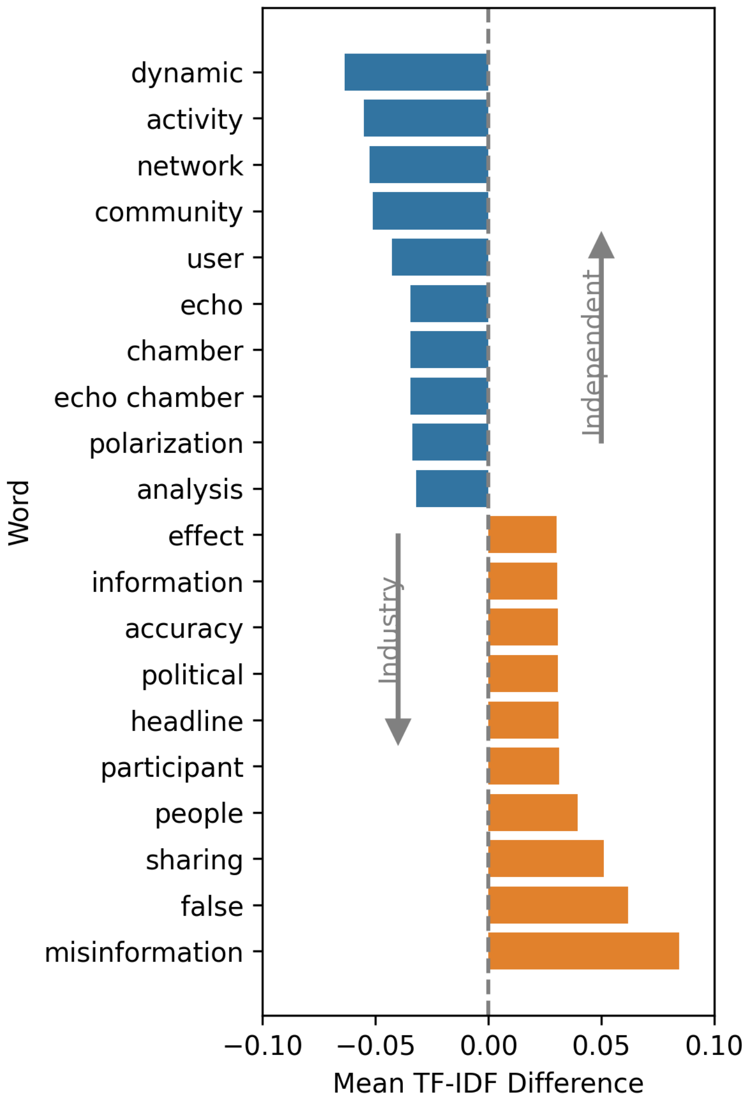


Figure S4: Top 10 distinct words for the industry-associated topic of misinformation sharing (bottom) and the independent work on platform dynamics (top).

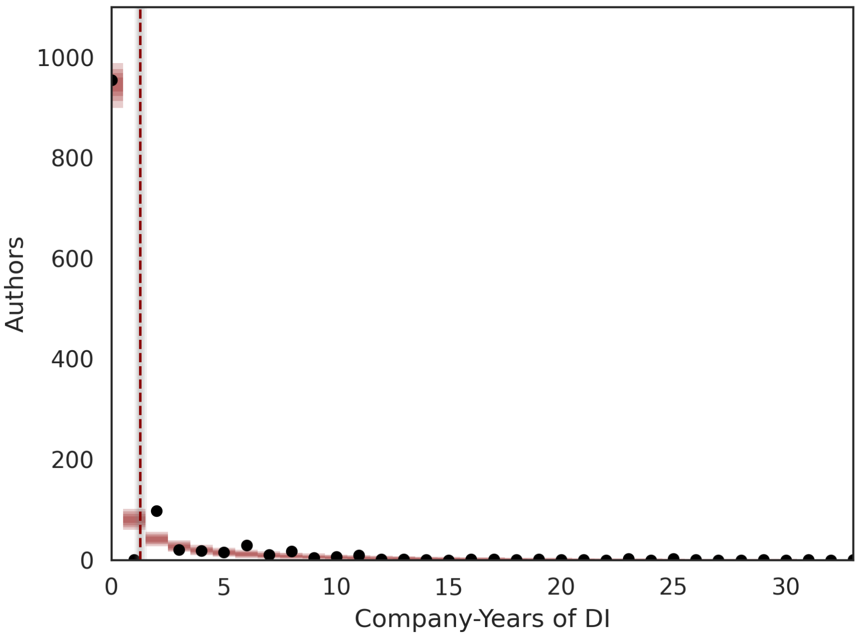


Figure S5: Posterior predictive distributions for our estimation of mean author-years of support. Shown are the actual and estimated density distributions. Dots indicate real values whereas shaded areas indicate posterior predictive distributions. Levels of opacity in the shading indicate the 50, 75, 89, 94, 97% credible regions. Note that the artifact at 1-2 years arises form our assumptions about funding/collaboration typically spanning more than a single year

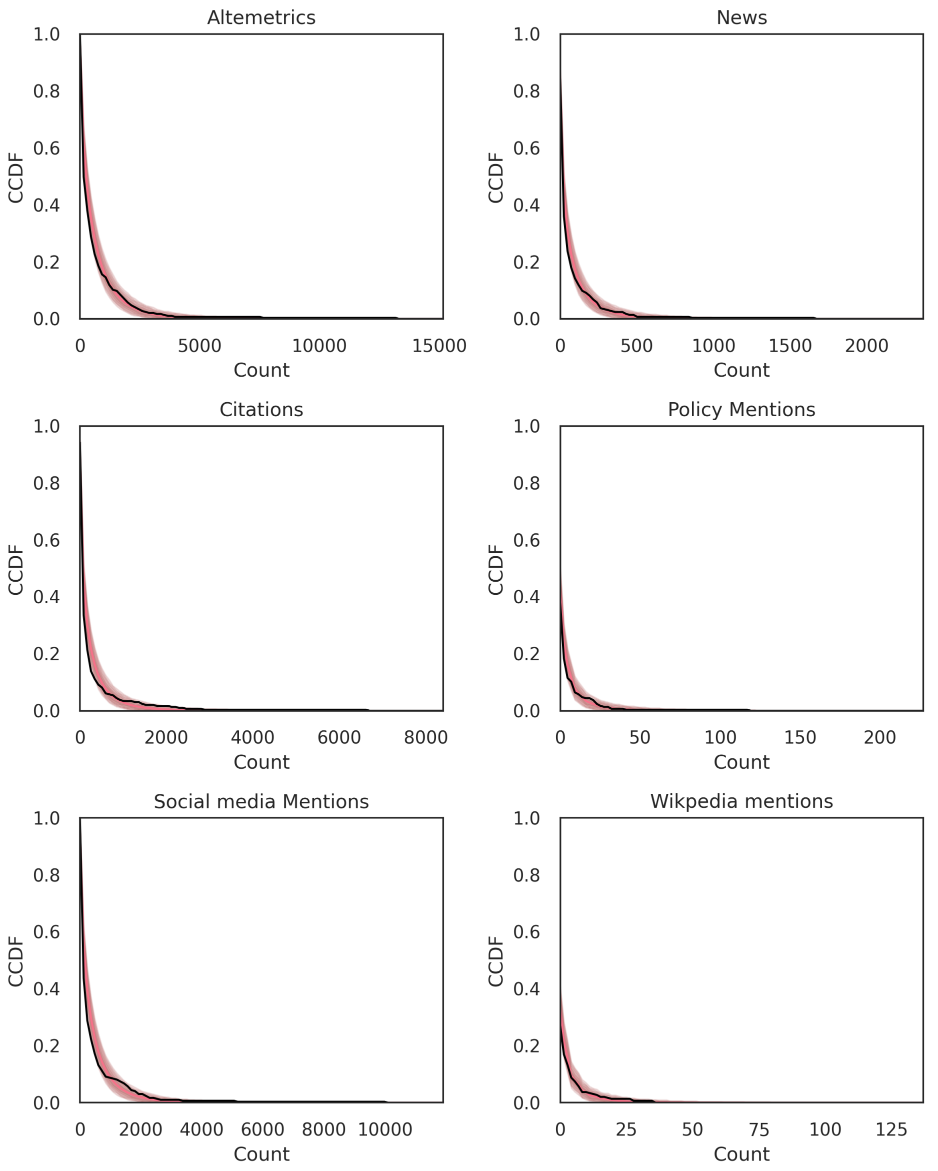


Figure S6: Posterior predictive distributions for all impact outcomes. Shown are the Complementary Cumulative Distribution Functions of the data (Black line) as well as the posterior predictive distributions as red shaded areas. Levels of opacity in the shading indicate the 50, 75, 89, 94, 97% credible regions.

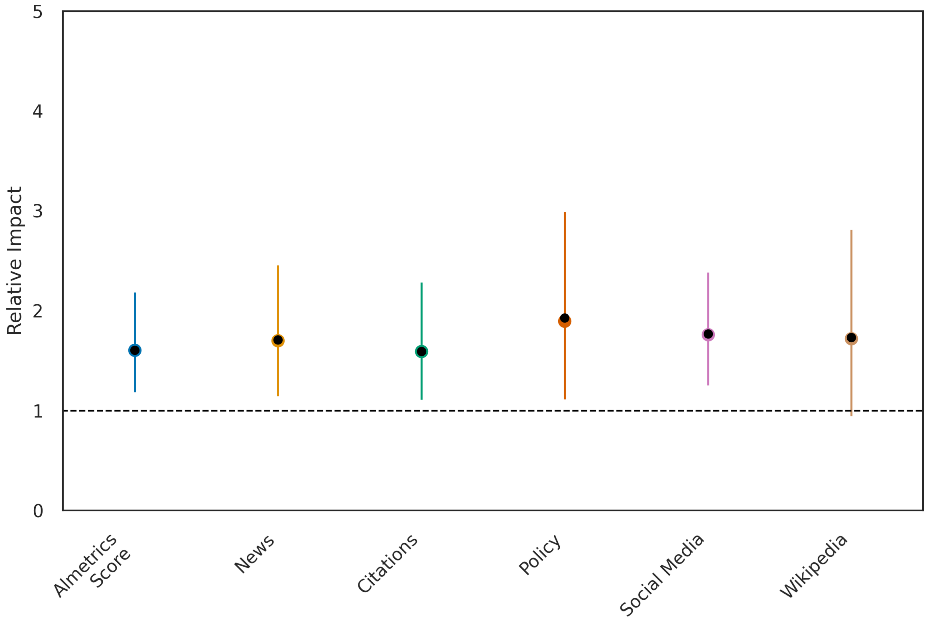


Figure S7: Relative impact as indicated in the main text, with black dots corresponding to the empirical mean impact to ensure the model is consistent with crude derived metrics from the data.

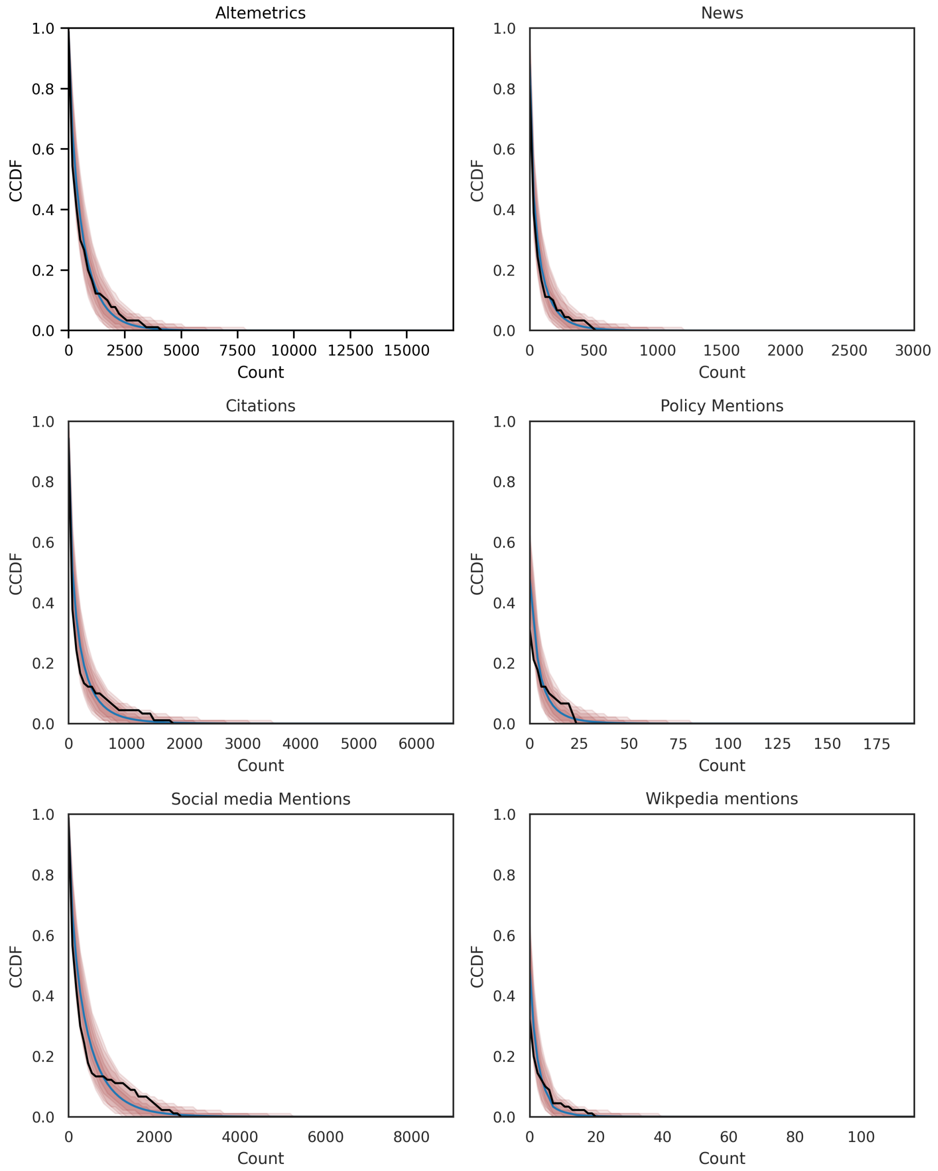


Figure S8: Posterior predictive distributions for all impact outcomes in our comparison of topics. Shown are the Complementary Cumulative Distribution Functions of the data (Black line) as well as the posterior predictive distributions as red shaded areas. Levels of opacity in the shading indicate the 50, 75, 89, 94, 97% credible regions.

## References

[1] Jason Priem, Heather Piwowar, and Rirchard Orr. "OpenAlex: A fully-open index of scholarly works, authors, venues, institutions, and concepts". In: *arXiv* (2022). arXiv: 2205.01833 [cs.DL]. URL: https://arxiv.org/abs/2205.01833.

[2] Aric Hagberg, Pieter J Swart, and Daniel A Schult. *Exploring network structure, dynamics, and function using NetworkX*. Tech. rep. Los Alamos National Laboratory (LANL), 2007.

[3] F. Pedregosa et al. "Scikit-learn: Machine Learning in Python". In: *Journal of Machine Learning Research* 12 (2011), pp. 2825–2830.

[4] Maarten Grootendorst. "BERTopic: Neural topic modeling with a class-based TF-IDF procedure". In: *arXiv preprint arXiv:2203.05794* (2022).

[5] Anand Patil, David Huard, and Christopher J Fonnesbeck. "PyMC: Bayesian stochastic modelling in Python". In: *Journal of statistical software* 35 (2010), pp. 1–81.
